# Supplementary material for: Transfer without Forgetting
Source: arXiv:2206.00388 source file (2022-07-25)
Supplement: Supplementary file 1 [file supp_att.tex]

% \begin{table}[ht]
%     \centering
% \caption{Final Average Accuracy (FAA) [$\uparrow$], Final Forgetting (FF) [$\downarrow$] and Average Accuracy Drop [$\downarrow$] (across buffer size w.r.t.\ the base method) of variants of \methnam trained on Split CIFAR-100 w.\ pre-train on Tiny ImageNet.}
%     \begin{tabular}{l@{\hskip 0.5cm}cc@{\hskip 0.5cm}cc}
%     \noalign{\smallskip}
%     \hline
%     \noalign{\smallskip}
%     \textbf{Variant}            & $|\mathcal{B}| = 500$  & $|\mathcal{B}| = 2000$ & Avg. Acc. Drop \\
%     \noalign{\smallskip}
%     \hline
%     \noalign{\smallskip}
%     No task conditioning        & \normres{54.63}{24.83} & \normres{63.19}{16.36} & $1.735$\\
%     $\mathbb{M}_\text{Sp}$ only & \normres{55.32}{25.37} & \normres{63.41}{16.30} & $1.280$\\
%     No $\mathbb{M}$             & \normres{55.77}{25.12} & \normres{63.12}{16.77} & $1.200$\\
%     No $\mathcal{L}_\text{AUX}$ & \normres{55.50}{24.99} & \normres{63.53}{16.03} & $1.130$\\
%     No $\mathbb{M}$ replay      & \normres{56.52}{25.12} & \normres{63.30}{16.31} & $0.735$\\
%     $\mathbb{M}_\text{Ch}$ only & \normres{56.49}{25.23} & \normres{63.50}{16.03} & $0.650$\\
%     \hline
%     \methnam           & \boldres{56.83}{23.89} & \boldres{64.46}{15.23} & -\\
%     \hline
%     \end{tabular}
%     \label{tab:att}
% \end{table}
